# Supplementary material for: A Proof of the Front-Door Adjustment Formula
Source: arXiv:1806.10449 ancillary file (2018-06-25)
Supplement: Supplementary file 1 [file frontDoorSlides.pdf]

# An Illustrated Proof of The Front-Door Adjustment Theorem

Mohammad Ali Javidian<sup>1</sup>   Marco Valtorta<sup>1</sup>

<sup>1</sup>Department of Computer Science  
University of South Carolina

June, 2018

# Outline

- 1 The Back-Door Criterion
  - Definition 1. (Back-Door)
  - Theorem 1. (Back-Door Adjustment)
- 2 The Front-Door Criterion
  - Definition 2. (Front-Door)
  - Theorem 2. (Front-Door Adjustment)
- 3 *do* Calculus
- 4 Proof of Theorem 2.

# Back-Door Criterion

## Definition

A set of variables  $Z$  satisfies the *back-door criterion* relative to an ordered pair of variables  $(X_i, X_j)$  in a DAG  $G$  if:

# Back-Door Criterion

## Definition

A set of variables  $Z$  satisfies the *back-door criterion* relative to an ordered pair of variables  $(X_i, X_j)$  in a DAG  $G$  if:

- (i) no node in  $Z$  is a descendant of  $X_i$ ; and

# Back-Door Criterion

## Definition

A set of variables  $Z$  satisfies the *back-door criterion* relative to an ordered pair of variables  $(X_i, X_j)$  in a DAG  $G$  if:

- (i) no node in  $Z$  is a descendant of  $X_i$ ; and
- (ii)  $Z$  blocks every path between  $X_i$  and  $X_j$  that contains an arrow into  $X_j$ .

## Definition 1. (Back-Door)

## Back-Door Criterion

## Definition

A set of variables  $Z$  satisfies the *back-door criterion* relative to an ordered pair of variables  $(X_i, X_j)$  in a DAG  $G$  if:

- (i) no node in  $Z$  is a descendant of  $X_i$ ; and
- (ii)  $Z$  blocks every path between  $X_i$  and  $X_j$  that contains an arrow into  $X_i$ .

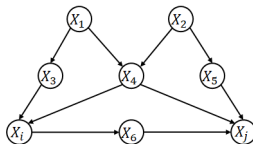

**Figure:**  $S_1 = \{X_3, X_4\}$  and  $S_2 = \{X_4, X_5\}$  would qualify under the back-door criterion, but  $S_3 = \{X_4\}$  would not because  $X_4$  does not  $d$ -separate  $X_i$  from  $X_j$  along the path  $(X_i, X_3, X_1, X_4, X_2, X_5, X_j)$ .

# Outline

- 1 The Back-Door Criterion
  - Definition 1. (Back-Door)
  - Theorem 1. (Back-Door Adjustment)
- 2 The Front-Door Criterion
  - Definition 2. (Front-Door)
  - Theorem 2. (Front-Door Adjustment)
- 3 *do* Calculus
- 4 Proof of Theorem 2.

# Back-Door Criterion

## Back-Door Adjustment Theorem

If a set of variables  $Z$  satisfies the back-door criterion relative to  $(X, Y)$ , then the causal effect of  $X$  on  $Y$  is identifiable and is given by the formula



# Back-Door Criterion

## Back-Door Adjustment Theorem

If a set of variables  $Z$  satisfies the back-door criterion relative to  $(X, Y)$ , then the causal effect of  $X$  on  $Y$  is identifiable and is given by the formula

$$P(y|\hat{x}) = \sum_z P(y|x, z)P(z). \quad (1)$$

# Outline

- 1 The Back-Door Criterion
  - Definition 1. (Back-Door)
  - Theorem 1. (Back-Door Adjustment)
- 2 The Front-Door Criterion
  - Definition 2. (Front-Door)
  - Theorem 2. (Front-Door Adjustment)
- 3 do Calculus
- 4 Proof of Theorem 2.

# Front-Door Criterion

## Definition

A set of variables  $Z$  satisfies the *front-door criterion* relative to an ordered pair of variables  $(X, Y)$  in a DAG  $G$  if:

# Front-Door Criterion

## Definition

A set of variables  $Z$  satisfies the *front-door criterion* relative to an ordered pair of variables  $(X, Y)$  in a DAG  $G$  if:

- (i)  $Z$  intercepts all directed paths from  $X$  to  $Y$ ;

# Front-Door Criterion

## Definition

A set of variables  $Z$  satisfies the *front-door criterion* relative to an ordered pair of variables  $(X, Y)$  in a DAG  $G$  if:

- (i)  $Z$  intercepts all directed paths from  $X$  to  $Y$ ;
- (ii) there is no unblocked back-door path from  $X$  to  $Z$ ; and

# Front-Door Criterion

## Definition

A set of variables  $Z$  satisfies the *front-door criterion* relative to an ordered pair of variables  $(X, Y)$  in a DAG  $G$  if:

- (i)  $Z$  intercepts all directed paths from  $X$  to  $Y$ ;
- (ii) there is no unblocked back-door path from  $X$  to  $Z$ ; and
- (iii) all back-door paths from  $Z$  to  $Y$  are blocked by  $X$ .

# Front-Door Criterion

## Definition

A set of variables  $Z$  satisfies the *front-door criterion* relative to an ordered pair of variables  $(X, Y)$  in a DAG  $G$  if:

- (i)  $Z$  intercepts all directed paths from  $X$  to  $Y$ ;
- (ii) there is no unblocked back-door path from  $X$  to  $Z$ ; and
- (iii) all back-door paths from  $Z$  to  $Y$  are blocked by  $X$ .

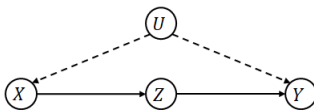

**Figure:** A diagram representing the front-door criterion.

# Outline

- 1 The Back-Door Criterion
  - Definition 1. (Back-Door)
  - Theorem 1. (Back-Door Adjustment)
- 2 The Front-Door Criterion
  - Definition 2. (Front-Door)
  - Theorem 2. (Front-Door Adjustment)
- 3 do Calculus
- 4 Proof of Theorem 2.



# Front-Door Criterion

## Front-Door Adjustment Theorem

If a set of variables  $Z$  satisfies the front-door criterion relative to  $(X, Y)$  and if  $P(x, z) > 0$ , then the causal effect of  $X$  on  $Y$  is identifiable and is given by the formula

## Theorem 2. (Front-Door Adjustment)

## Front-Door Criterion

## Front-Door Adjustment Theorem

If a set of variables  $Z$  satisfies the front-door criterion relative to  $(X, Y)$  and if  $P(x, z) > 0$ , then the causal effect of  $X$  on  $Y$  is identifiable and is given by the formula

$$P(y|\hat{x}) = \sum_z P(z|x) \sum_{x'} P(y|x', z) P(x').$$

# Rules of *do* Calculus

## Preliminary Notation

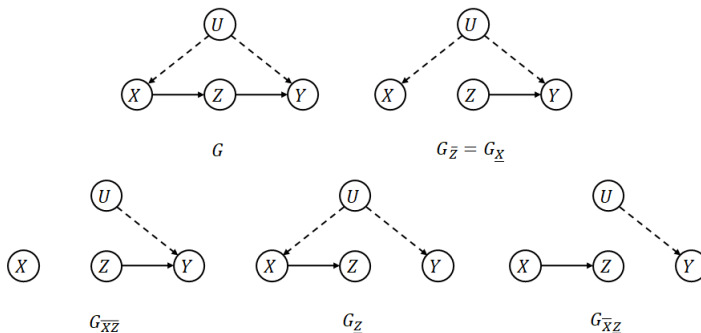

**Figure:** Subgraphs of  $G$  used in the derivation of causal effects.

# Inference Rules

## Rules of *do* Calculus

**Rule 1** (Insertion/deletion of observations):

$$P(y|\hat{x}, z, w) = P(y|\hat{x}, w) \quad \text{if} \quad (Y \perp\!\!\!\perp Z|X, W)_{G_{\bar{X}}}.$$

# Inference Rules

## Rules of *do* Calculus

**Rule 1** (Insertion/deletion of observations):

$$P(y|\hat{x}, z, w) = P(y|\hat{x}, w) \quad \text{if} \quad (Y \perp\!\!\!\perp Z|X, W)_{G_{\bar{X}}}.$$

**Rule 2** (Action/observation exchange):

$$P(y|\hat{x}, \hat{z}, w) = P(y|\hat{x}, z, w) \quad \text{if} \quad (Y \perp\!\!\!\perp Z|X, W)_{G_{\bar{X}\bar{Z}}}.$$

# Inference Rules

## Rules of *do* Calculus

**Rule 1** (Insertion/deletion of observations):

$$P(y|\hat{x}, z, w) = P(y|\hat{x}, w) \quad \text{if} \quad (Y \perp\!\!\!\perp Z|X, W)_{G_{\overline{X}}}.$$

**Rule 2** (Action/observation exchange):

$$P(y|\hat{x}, \hat{z}, w) = P(y|\hat{x}, z, w) \quad \text{if} \quad (Y \perp\!\!\!\perp Z|X, W)_{G_{\overline{X}, \underline{Z}}}.$$

**Rule 3** (Insertion/deletion of actions):

$$P(y|\hat{x}, \hat{z}, w) = P(y|\hat{x}, w) \quad \text{if} \quad (Y \perp\!\!\!\perp Z|X, W)_{G_{\overline{X}, \overline{Z(W)}}}.$$

where  $Z(W)$  is the set of  $Z$ -nodes that are not ancestors of any  $W$ -node in  $G_{\overline{X}}$ .

# Proof of Front-Door Adjustment Theorem

Step 1: Compute  $P(z|\hat{x})$

- $X \perp\!\!\!\perp Z$  in  $G_{\underline{X}}$  because there is no outgoing edge from  $X$  in  $G_{\underline{X}}$ , and also by condition (ii) of the definition of the front-door criterion, all back-door paths from  $X$  to  $Z$  are blocked.

Step 1: Compute  $P(z|\hat{x})$

-



# Proof of Front-Door Adjustment Theorem

## Step 1: Compute $P(z|\hat{x})$

- $X \perp\!\!\!\perp Z$  in  $G_{\underline{X}}$  because there is no outgoing edge from  $X$  in  $G_{\underline{X}}$ , and also by condition (ii) of the definition of the front-door criterion, all back-door paths from  $X$  to  $Z$  are blocked.

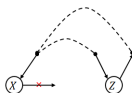

- $G$  satisfies the applicability condition for Rule 2:

$$P(y|\hat{x}, \hat{z}, w) = P(y|\hat{x}, z, w) \quad \text{if} \quad (Y \perp\!\!\!\perp Z|X, W)_{G_{\overline{XZ}}}.$$

# Proof of Front-Door Adjustment Theorem

## Step 1: Compute $P(z|\hat{x})$

- $X \perp\!\!\!\perp Z$  in  $G_{\underline{X}}$  because there is no outgoing edge from  $X$  in  $G_{\underline{X}}$ , and also by condition (ii) of the definition of the front-door criterion, all back-door paths from  $X$  to  $Z$  are blocked.

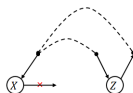

- $G$  satisfies the applicability condition for Rule 2:

$$P(y|\hat{x}, \hat{z}, w) = P(y|\hat{x}, z, w) \quad \text{if} \quad (Y \perp\!\!\!\perp Z|X, W)_{G_{\overline{XZ}}}.$$

- In Rule 2, set  $y = z, x = \emptyset, z = x, w = \emptyset$ :

# Proof of Front-Door Adjustment Theorem

Step 1: Compute  $P(z|\hat{x})$

- $X \perp\!\!\!\perp Z$  in  $G_{\underline{X}}$  because there is no outgoing edge from  $X$  in  $G_{\underline{X}}$ , and also by condition (ii) of the definition of the front-door criterion, all back-door paths from  $X$  to  $Z$  are blocked.

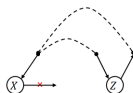

- $G$  satisfies the applicability condition for Rule 2:

$$P(y|\hat{x}, \hat{z}, w) = P(y|\hat{x}, z, w) \quad \text{if} \quad (Y \perp\!\!\!\perp Z|X, W)_{G_{\overline{XZ}}}.$$

- In Rule 2, set  $y = z, x = \emptyset, z = x, w = \emptyset$ :

$$P(z|\hat{x}) = P(z|x) \quad \text{because} \quad (Z \perp\!\!\!\perp X)_{G_{\underline{X}}}.$$

# Proof of Front-Door Adjustment Theorem

Step 2: Compute  $P(y|\hat{z})$

- $P(y|\hat{z}) = \sum_x P(y|x, \hat{z})P(x|\hat{z}).$

# Proof of Front-Door Adjustment Theorem

## Step 2: Compute $P(y|\hat{z})$

- $P(y|\hat{z}) = \sum_x P(y|x, \hat{z})P(x|\hat{z})$ .
- $X \perp\!\!\!\perp Z$  in  $G_{\bar{Z}}$  because there is no incoming edge to  $Z$  in  $G_{\bar{Z}}$ , and also all paths from  $X$  to  $Z$  either by condition (ii) of the definition of the front-door criterion (blue-type paths), or because of existence of a collider node on the path (green-type paths) are blocked.

# Proof of Front-Door Adjustment Theorem

## Step 2: Compute $P(y|\hat{z})$

- $P(y|\hat{z}) = \sum_x P(y|x, \hat{z})P(x|\hat{z})$ .
- $X \perp\!\!\!\perp Z$  in  $G_{\bar{Z}}$  because there is no incoming edge to  $Z$  in  $G_{\bar{Z}}$ , and also all paths from  $X$  to  $Z$  either by condition (ii) of the definition of the front-door criterion (blue-type paths), or because of existence of a collider node on the path (green-type paths) are blocked.

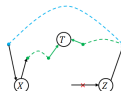

# Proof of Front-Door Adjustment Theorem

## Step 2: Compute $P(y|\hat{z})$

- $P(y|\hat{z}) = \sum_x P(y|x, \hat{z})P(x|\hat{z})$ .
- $X \perp\!\!\!\perp Z$  in  $G_{\bar{Z}}$  because there is no incoming edge to  $Z$  in  $G_{\bar{Z}}$ , and also all paths from  $X$  to  $Z$  either by condition (ii) of the definition of the front-door criterion (blue-type paths), or because of existence of a collider node on the path (green-type paths) are blocked.

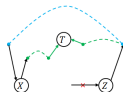

- $G$  satisfies the applicability condition for Rule 3:

$$P(y|\hat{x}, \hat{z}, w) = P(y|\hat{x}, w) \quad \text{if} \quad (Y \perp\!\!\!\perp Z|X, W)_{G_{\bar{X}, \bar{Z}(w)}}.$$

# Proof of Front-Door Adjustment Theorem

## Step 2: Compute $P(y|\hat{z})$

- $P(y|\hat{z}) = \sum_x P(y|x, \hat{z})P(x|\hat{z})$ .
- $X \perp\!\!\!\perp Z$  in  $G_{\overline{Z}}$  because there is no incoming edge to  $Z$  in  $G_{\overline{Z}}$ , and also all paths from  $X$  to  $Z$  either by condition (ii) of the definition of the front-door criterion (blue-type paths), or because of existence of a collider node on the path (green-type paths) are blocked.

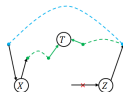

- $G$  satisfies the applicability condition for Rule 3:

$$P(y|\hat{x}, \hat{z}, w) = P(y|\hat{x}, w) \quad \text{if} \quad (Y \perp\!\!\!\perp Z | X, W)_{G_{\overline{X}, \overline{Z}(W)}}.$$

- In Rule 3, set  $y = x, x = \emptyset, z = z, w = \emptyset$ :



# Proof of Front-Door Adjustment Theorem

## Step 2: Compute $P(y|\hat{z})$

- $P(y|\hat{z}) = \sum_x P(y|x, \hat{z})P(x|\hat{z})$ .
- $X \perp\!\!\!\perp Z$  in  $G_{\overline{Z}}$  because there is no incoming edge to  $Z$  in  $G_{\overline{Z}}$ , and also all paths from  $X$  to  $Z$  either by condition (ii) of the definition of the front-door criterion (blue-type paths), or because of existence of a collider node on the path (green-type paths) are blocked.

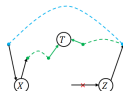

- $G$  satisfies the applicability condition for Rule 3:

$$P(y|\hat{x}, \hat{z}, w) = P(y|\hat{x}, w) \quad \text{if} \quad (Y \perp\!\!\!\perp Z | X, W)_{G_{\overline{X}, \overline{Z(W)}}}.$$

- In Rule 3, set  $y = x, x = \emptyset, z = z, w = \emptyset$ :

$$P(x|\hat{z}) = P(x) \quad \text{because} \quad (Z \perp\!\!\!\perp X)_{G_{\overline{Z}}}.$$

# Proof of Front-Door Adjustment Theorem

Step 2 (continued): Compute  $P(y|\hat{z})$

- $(Z \perp\!\!\!\perp Y|X)_{G_{\underline{Z}}}$  because there is no outgoing edge from  $Z$  in  $G_{\underline{Z}}$ , and also by condition (iii) of the definition of the front-door criterion, all back-door paths from  $Z$  to  $Y$  are blocked by  $X$ .

# Proof of Front-Door Adjustment Theorem

Step 2 (continued): Compute  $P(y|\hat{z})$

- $(Z \perp\!\!\!\perp Y|X)_{G_{\underline{Z}}}$  because there is no outgoing edge from  $Z$  in  $G_{\underline{Z}}$ , and also by condition (iii) of the definition of the front-door criterion, all back-door paths from  $Z$  to  $Y$  are blocked by  $X$ .

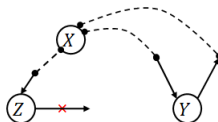

# Proof of Front-Door Adjustment Theorem

Step 2 (continued): Compute  $P(y|\hat{z})$

- $(Z \perp\!\!\!\perp Y|X)_{G_{\underline{Z}}}$  because there is no outgoing edge from  $Z$  in  $G_{\underline{Z}}$ , and also by condition (iii) of the definition of the front-door criterion, all back-door paths from  $Z$  to  $Y$  are blocked by  $X$ .

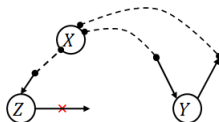

- $G$  satisfies the applicability condition for Rule 2:  
 $P(y|\hat{x}, \hat{z}, w) = P(y|\hat{x}, z, w)$  if  $(Y \perp\!\!\!\perp Z|X, W)_{G_{\overline{X}\underline{Z}}}$ .

# Proof of Front-Door Adjustment Theorem

Step 2 (continued): Compute  $P(y|\hat{z})$

- $(Z \perp\!\!\!\perp Y|X)_{G_{\underline{Z}}}$  because there is no outgoing edge from  $Z$  in  $G_{\underline{Z}}$ , and also by condition (iii) of the definition of the front-door criterion, all back-door paths from  $Z$  to  $Y$  are blocked by  $X$ .

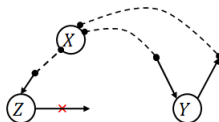

- $G$  satisfies the applicability condition for Rule 2:  
 $P(y|\hat{x}, \hat{z}, w) = P(y|\hat{x}, z, w)$  if  $(Y \perp\!\!\!\perp Z|X, W)_{G_{\overline{X\hat{Z}}}}$ .
- In Rule 2, set  $y = y, x = \emptyset, z = z, w = x$ :

# Proof of Front-Door Adjustment Theorem

Step 2 (continued): Compute  $P(y|\hat{z})$

- $(Z \perp\!\!\!\perp Y|X)_{G_{\underline{Z}}}$  because there is no outgoing edge from  $Z$  in  $G_{\underline{Z}}$ , and also by condition (iii) of the definition of the front-door criterion, all back-door paths from  $Z$  to  $Y$  are blocked by  $X$ .

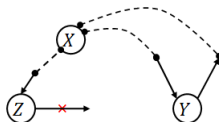

- $G$  satisfies the applicability condition for Rule 2:  
 $P(y|\hat{x}, \hat{z}, w) = P(y|\hat{x}, z, w)$  if  $(Y \perp\!\!\!\perp Z|X, W)_{G_{\overline{X}\underline{Z}}}$ .
- In Rule 2, set  $y = y, x = \emptyset, z = z, w = x$ :

$$P(y|x, \hat{z}) = P(y|x, z) \quad \text{because} \quad (Z \perp\!\!\!\perp Y|X)_{G_{\underline{Z}}}.$$

# Proof of Front-Door Adjustment Theorem

Step 2 (continued): Compute  $P(y|\hat{z})$

- $$P(y|\hat{z}) = \sum_x P(y|x, \hat{z})P(x|\hat{z}) = \sum_x P(y|x, z)P(x).$$

# Proof of Front-Door Adjustment Theorem

Step 2 (continued): Compute  $P(y|\hat{z})$

- $P(y|\hat{z}) = \sum_x P(y|x, \hat{z})P(x|\hat{z}) = \sum_x P(y|x, z)P(x).$
- This formula is a special case of the back-door formula in Theorem 1.



# Proof of Front-Door Adjustment Theorem

Step 3: Compute  $P(y|\hat{x})$

- $P(y|\hat{x}) = \sum_z P(y|z, \hat{x})P(z|\hat{x}).$

# Proof of Front-Door Adjustment Theorem

Step 3: Compute  $P(y|\hat{x})$

- $P(y|\hat{x}) = \sum_z P(y|z, \hat{x})P(z|\hat{x})$ .
- $(Y \perp\!\!\!\perp Z|X)_{G_{\overline{XZ}}}$  because there is no outgoing edge from  $Z$  in  $G_{\overline{XZ}}$ , and also by condition (iii) of the definition of the front-door criterion, all back-door paths from  $Z$  to  $Y$  are blocked by  $X$ .

Step 3: Compute  $P(y|\hat{x})$

- $P(y|\hat{x}) = \sum_z P(y|z, \hat{x})P(z|\hat{x})$ .
- $(Y \perp\!\!\!\perp Z|X)_{G_{\overline{XZ}}}$  because there is no outgoing edge from  $Z$  in  $G_{\overline{XZ}}$ , and also by condition (iii) of the definition of the front-door criterion, all back-door paths from  $Z$  to  $Y$  are blocked by  $X$ .

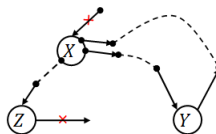

# Proof of Front-Door Adjustment Theorem

## Step 3: Compute $P(y|\hat{x})$

- $P(y|\hat{x}) = \sum_z P(y|z, \hat{x})P(z|\hat{x})$ .
- $(Y \perp\!\!\!\perp Z|X)_{G_{\overline{XZ}}}$  because there is no outgoing edge from  $Z$  in  $G_{\overline{XZ}}$ , and also by condition (iii) of the definition of the front-door criterion, all back-door paths from  $Z$  to  $Y$  are blocked by  $X$ .

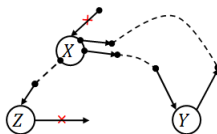

- $G$  satisfies the applicability condition for Rule 2:  
 $P(y|\hat{x}, \hat{z}, w) = P(y|\hat{x}, z, w) \quad \text{if} \quad (Y \perp\!\!\!\perp Z|X, W)_{G_{\overline{XZ}}}.$

# Proof of Front-Door Adjustment Theorem

## Step 3: Compute $P(y|\hat{x})$

- $P(y|\hat{x}) = \sum_z P(y|z, \hat{x})P(z|\hat{x})$ .
- $(Y \perp\!\!\!\perp Z|X)_{G_{\overline{XZ}}}$  because there is no outgoing edge from  $Z$  in  $G_{\overline{XZ}}$ , and also by condition (iii) of the definition of the front-door criterion, all back-door paths from  $Z$  to  $Y$  are blocked by  $X$ .

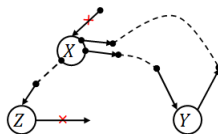

- $G$  satisfies the applicability condition for Rule 2:  
 $P(y|\hat{x}, \hat{z}, w) = P(y|\hat{x}, z, w) \quad \text{if} \quad (Y \perp\!\!\!\perp Z|X, W)_{G_{\overline{XZ}}}.$
- In Rule 2, set  $y = y, x = \hat{x}, z = z, w = \emptyset$  :

# Proof of Front-Door Adjustment Theorem

## Step 3: Compute $P(y|\hat{x})$

- $P(y|\hat{x}) = \sum_z P(y|z, \hat{x})P(z|\hat{x})$ .
- $(Y \perp\!\!\!\perp Z|X)_{G_{\overline{XZ}}}$  because there is no outgoing edge from  $Z$  in  $G_{\overline{XZ}}$ , and also by condition (iii) of the definition of the front-door criterion, all back-door paths from  $Z$  to  $Y$  are blocked by  $X$ .

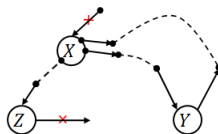

- $G$  satisfies the applicability condition for Rule 2:  
 $P(y|\hat{x}, \hat{z}, w) = P(y|\hat{x}, z, w) \quad \text{if} \quad (Y \perp\!\!\!\perp Z|X, W)_{G_{\overline{XZ}}}.$
- In Rule 2, set  $y = y, x = \hat{x}, z = z, w = \emptyset$ :

$$P(y|z, \hat{x}) = P(y|\hat{z}, \hat{x}) \quad \text{because} \quad (Y \perp\!\!\!\perp Z|X)_{G_{\overline{XZ}}}.$$

# Proof of Front-Door Adjustment Theorem

Step 3 (continued): Compute  $P(y|\hat{x})$

- $(Y \perp\!\!\!\perp X|Z)_{G_{\overline{XZ}}}$  because there is no incoming edge to  $X$  in  $G_{\overline{XZ}}$ , and also all paths from  $X$  to  $Y$  are blocked either because of condition (i) of the definition of the front-door criterion (blue-type paths)[directed paths from  $X$  to  $Y$ ], or because of the existence of a collider on the path (green-type paths) (note that the case  $T \in Z$  cannot happen because there is no incoming edge to  $Z$  in  $G_{\overline{XZ}}$ ).

# Proof of Front-Door Adjustment Theorem

Step 3 (continued): Compute  $P(y|\hat{x})$

- $(Y \perp\!\!\!\perp X|Z)_{G_{\overline{XZ}}}$  because there is no incoming edge to  $X$  in  $G_{\overline{XZ}}$ , and also all paths from  $X$  to  $Y$  are blocked either because of condition (i) of the definition of the front-door criterion (blue-type paths)[directed paths from  $X$  to  $Y$ ], or because of the existence of a collider on the path (green-type paths) (note that the case  $T \in Z$  cannot happen because there is no incoming edge to  $Z$  in  $G_{\overline{XZ}}$ ).

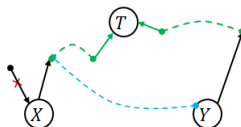



# Proof of Front-Door Adjustment Theorem

Step 3 (continued): Compute  $P(y|\hat{x})$

- $G$  satisfies the applicability condition for Rule 3:

$$P(y|\hat{x}, \hat{z}, w) = P(y|\hat{x}, w) \quad \text{if} \quad (Y \perp\!\!\!\perp Z|X, W)_{G_{\overline{X}, \overline{Z(W)}}}.$$

# Proof of Front-Door Adjustment Theorem

Step 3 (continued): Compute  $P(y|\hat{x})$

- $G$  satisfies the applicability condition for Rule 3:

$$P(y|\hat{x}, \hat{z}, w) = P(y|\hat{x}, w) \quad \text{if} \quad (Y \perp\!\!\!\perp Z | X, W)_{G_{\overline{X}, \overline{Z(w)}}}.$$

- In Rule 3, set  $y = y, x = z, z = x, w = \emptyset$ :

# Proof of Front-Door Adjustment Theorem

Step 3 (continued): Compute  $P(y|\hat{x})$

- $G$  satisfies the applicability condition for Rule 3:

$$P(y|\hat{x}, \hat{z}, w) = P(y|\hat{x}, w) \quad \text{if} \quad (Y \perp\!\!\!\perp Z|X, W)_{G_{\overline{X, \overline{Z(w)}}}}.$$

- In Rule 3, set  $y = y, x = z, z = x, w = \emptyset$ :

$$P(y|\hat{z}, \hat{x}) = P(y|\hat{z}) \quad \text{because} \quad (Y \perp\!\!\!\perp Z|X)_{G_{\overline{XZ}}}.$$

# Proof of Front-Door Adjustment Theorem

Step 3 (continued): Compute  $P(y|\hat{x})$

- $G$  satisfies the applicability condition for Rule 3:

$$P(y|\hat{x}, \hat{z}, w) = P(y|\hat{x}, w) \quad \text{if} \quad (Y \perp\!\!\!\perp Z|X, W)_{G_{\overline{X}, \overline{Z(W)}}}.$$

- In Rule 3, set  $y = y, x = z, z = x, w = \emptyset$ :

$$P(y|\hat{z}, \hat{x}) = P(y|\hat{z}) \quad \text{because} \quad (Y \perp\!\!\!\perp Z|X)_{G_{\overline{XZ}}}.$$

- $P(y|\hat{x}) = \sum_z P(y|z, \hat{x})P(z|\hat{x}) = \sum_z P(z|x) \sum_{x'} P(y|x', z)P(x').$

# Reference For Further Reading

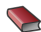

J. Pearl.

*Causality. Models, reasoning, and inference.*

Cambridge University Press, 2009.
